# Supplementary material for: Anisotropic melting of frustrated Ising antiferromagnets
Source: arXiv:2112.15514 source file (2021-12-31)
Supplement: Supplementary file 1 [file supplement_compiled.pdf]

# Supplementary Material for *Anisotropic Melting of Frustrated Ising Antiferromagnets*

(Dated: December 31, 2021)

## MONTE CARLO METHOD

### Local and Cluster Updates

The cluster update algorithm was based on the Wolff method [1], with the Luijten-Blöte [2] modification for long-range interactions. Additionally, the activation probability of a given bond was changed from $p(\sigma_i, \sigma_j) = \delta_{\sigma_i \sigma_j}(1-e^{-K})$ to $p'(\sigma_i, \sigma_j) = \Theta(-K\sigma_i\sigma_j)(1 - e^{-|K|})$, where $K = \beta J_{ij}$ and $\Theta(x)$ is the Heaviside step function. In essence, this modification accounts for mixed-sign interactions by still selecting spins that are aligned favorably with one another according to their respective interactions. The Monte Carlo sign problem is still present, due to frustration, so parallel tempering is incorporated (See the following section), with replicas in a grid of 16 different values of $T$ for each simulation. All simulations were performed with $L_x = L_z = 64$, with some consistency checks with $L_x = L_z = 32$ and $L_x = L_z = 120$ to ensure that the results are not sensitive to the finite-size effects. Outside of the LRO phase with $J_{z2} \geq 0.5 J_{z1}$, good convergence was typically achieved with $10^6$ measurements, with 100 Metropolis steps and 1 Wolff step per measurement, and a parallel tempering step every 10 measurements.

### Parallel Tempering

Parallel tempering is a Monte Carlo technique that uses replicas of a frustrated system at different temperatures to facilitate stochastic movement out of local minima in the energy landscape. This technique was developed to study spin glasses [3–5] but can be used fruitfully in other frustrated models as well [6]. A single calculation usually includes multiple copies of a system running in parallel with their own local updates, performed at a grid of different temperatures. The parallel tempering update then swaps the systems at different temperatures according to an appropriate acceptance probability.

Suppose there are two systems $\mu$ and $\nu$, running in parallel, with inverse temperatures $\beta_1$ and $\beta_2$, respectively, and energies $E_\mu$ and $E_\nu$. To swap between the microstates $\mu$ and $\nu$ while satisfying detailed balance at a fixed temperature $\beta$, one must choose an acceptance probability

$$\frac{P(\mu \to \nu, \beta)}{P(\nu \to \mu, \beta)} = e^{\beta(E_\mu - E_\nu)}. \tag{1}$$

Therefore, in the example with the parallel systems at $\beta_1$ and $\beta_2$, a swap of the two microstates must satisfy

$$\begin{aligned} \frac{P(\mu \to \nu, \beta_1)}{P(\nu \to \mu, \beta_1)} \frac{P(\nu \to \mu, \beta_2)}{P(\mu \to \nu, \beta_2)} &= e^{\beta_1(E_\mu - E_\nu) + \beta_2(E_\nu - E_\mu)} \\ &= e^{(\beta_1 - \beta_2)(E_\mu - E_\nu)}. \end{aligned} \tag{2}$$

In the simulations used for the main text, a typical calculation includes a grid of 16 values of $\beta$, with the parallel tempering update occurring after 1000 Metropolis steps, 10 cluster updates, and 10 measurement steps. In the parallel tempering update, the systems at adjacent temperatures are proposed to swap with probabilities given by the condition in Eq. 2. The swap proposals continue for every pair of microstates that are adjacent in temperature, starting with the lowest value of $\beta$ (highest temperature).

## SPIN CORRELATION FUNCTIONS

The lattice momentum $q$ can be commensurate with values $Q_1 \equiv \pi$ or $Q_2 \equiv \frac{\pi}{2}$, or incommensurate with $q$ continuously varying between $\frac{\pi}{2}$ and $\pi$. The momenta denoted by capital letters ($Q_1$, $Q_2$) denote LRO while the lower-case $q$ denotes a variable momentum at which the structure factor is maximized in the SRO or floating phases.

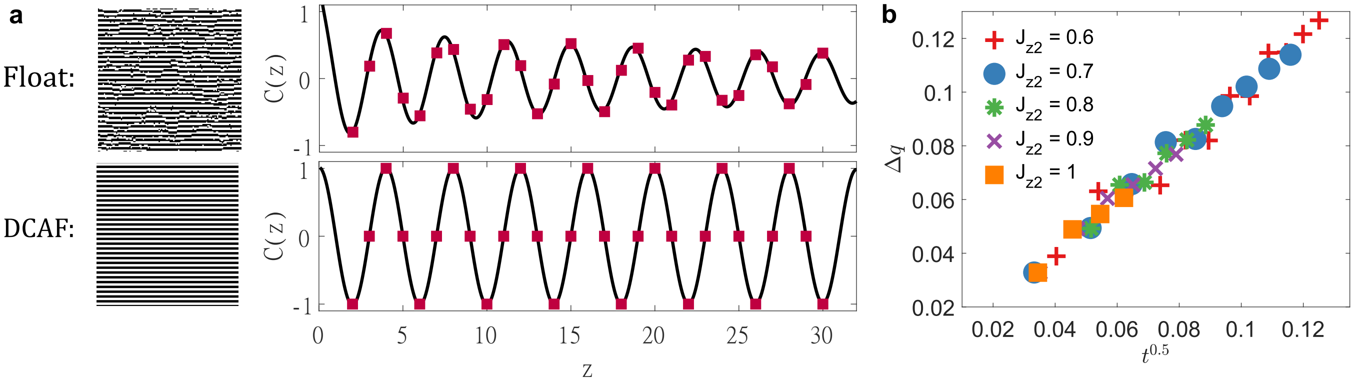


FIG. 1. **(a)** Bitmap images of the spins in the indicated phases and their resulting microstate correlation functions $C(z) = L^{-2}\sum_{\mathbf{r}} \sigma(\mathbf{r})\sigma(\mathbf{r}+z)$. The solid black line is a fit to the Ornstein-Zernike form $C(z) \sim z^{-\eta}\exp(-z/\xi)\cos(qz)$, with $\eta$, $\xi$, and $q$ as fit parameters. The floating phase can be visually recognized by a distinctive pattern of domain boundaries that stretch across the system. **(b)** Data collapse of the degree of incommensurability vs. the scaled reduced temperature $t = \frac{T-T_c}{T_c}$, demonstrating the power law $\Delta q \sim t^{\beta}$ with $\beta = 0.5$.

Aside from commensurate (C) vs. incommensurate (IC), the decay profile further specifies a given phase. The three possible decay profiles are

$$\begin{cases} C(r) \sim \cos(qr)\frac{\exp(-r/\xi)}{\sqrt{r}} & \text{Short-range Order (SRO)} \\ C(r) \sim \cos(qr)\frac{1}{r^{\eta}} & \text{Floating, } 0 < \eta < 1/4 \\ C(r) \sim \cos(Qr) & \text{Antiferro (AF), } Q = (Q_1 \text{ or } Q_2) \end{cases} \tag{3}$$

The short-range phases have commensurate (C-SRO) or incommensurate (IC-SRO) correlations. In the regime of weak frustration $J_{z2} \lesssim J_{z1}/2$, the low-temperature ordered phase is the Column Antiferromagnet (CAF) with $\mathbf{Q}_1 = (0, \pi)$.

## TRANSITION FROM FLOATING PHASE TO DCAF PHASE

The floating phase is analogous to the quasi-long-range ordered phase found in the XY model [7]. However, the transition to the DCAF phase does not have a true analogue in the BKT theory, because there is no true long-range order in the two-dimensional XY model [8]. This transition turns out to be second-order, with the typical power law scaling that can be most easily seen in the degree of incommensurability, $\Delta q$, because the correlation length is infinite in both phases. This scaling is illustrated in Fig. 1(b), along with Monte Carlo snapshots and the resulting correlation functions for the two phases.

## DATA FOR $J_{z1} = 0.1|J_0|$

Additional data for the weak inter-chain coupling $J_{z1} = 0.1|J_0|$ is shown in Fig. 2. The primary result is the nearly constant value of $T^*$ shown in panel (b), which further demonstrates that $T^*$ depends mainly on the mean field energy scales of the problem. Specifically, the magnitude of $J_0$ dominates in this regime so frustration does not suppress $T^*$ as much as in the case $J_{z1} = |J_0|$.

## LIFSHITZ AND DISORDER TRANSITIONS

Figure 3 demonstrates the distinctions between $T_N$, $T_L$, and $T_D$ within the ANNNI phase diagram. For fixed values of $J_{z2}$ near the frustration point $J_{z2} = 0.5J_{z1}$, an increase in temperature melts the CAF order almost immediately into the incommensurate paramagnetic phase; this means the Néel temperature and the disorder/Lifshitz transition [9] are very close for high levels of frustration. When the fixed $J_{z2}$ is small ($\sim 0.1J_{z1}$), an increase in temperature leads

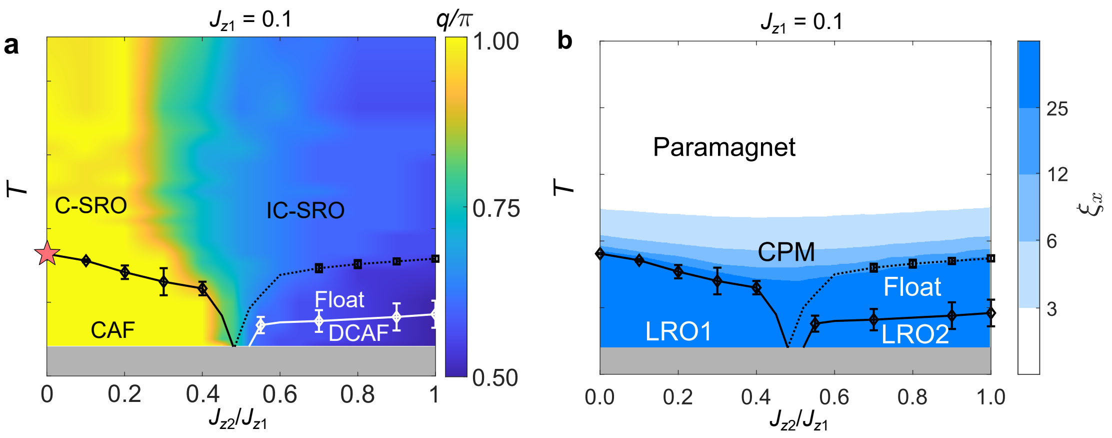


FIG. 2. **(a)** False color plot of the dominant ordering wavevector in $T$-$J_{z2}$ parameter space for $J_{z1} = 0.1$. The overall features are similar to those described in the main text. **(b)** Contour plot of the droplet size in $T$-$J_{z2}$ parameter space for $J_{z1} = 0.1$. Here, $T^*$ is determined almost entirely by the scale of the interactions in the $x$-dimension ($J_0$).

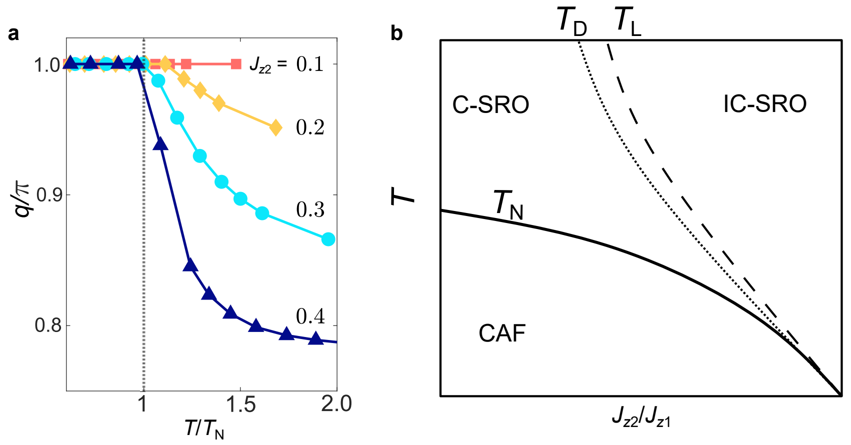


FIG. 3. **(a)** Dominant wavevector $q$ in the correlations at different values of $J_{z2}$, as a function of temperature. The wavevector differs from $\pi$ more significantly as frustration is increased $J_{z2} \to 0.5$ and as temperature is increased. For weaker frustration the deviation in $q$ appears at larger and larger proportions of the Néel temperature. **(b)** Sketch of the distinction between Lifshitz ($T_L$) and Disorder ($T_D$) temperatures. At fixed temperature, with increasing $J_{z2}$, first the correlation length has a kink as is switches from decreasing to increasing at $T_D$ [9]. At $T_L$, the Fourier-space correlations develop a double-peak structure which is the signature of the incommensurate phases described in the main text.

the CAF order to melt directly into the commensurate ($q = \pi$) paramagnetic phase. The Lifshitz temperature becomes vertical in the infinite-$T$ limit, as shown by the color gradient in Fig. 2(a).

The distinction between disorder and Lifshitz temperatures manifests in the real-space correlations and the Fourier-space correlations, respectively [9]. At the disorder transition ($T_D$), with fixed $T$ and increasing $J_{z2}$, the (real-space) correlation length experiences a local minimum with a kink. The C-SRO phase then persists until the system reaches the Lifshitz transition ($T_L$). At the Lifshitz transition, the Fourier-space correlation function shifts from a single-peaked structure centered at $q = \pi$ to a double-peaked structure with peaks at $q = \pi \pm \Delta q$. These features are illustrated and discussed in the main text. The Lifshitz transition is the only one discussed in the main text because the signature is more intuitive and in practice the two transitions occur so close together they are impossible to distinguish on the scales studied.

[1] U. Wolff, Collective Monte Carlo updating for spin systems, Phys. Rev. Lett. **62**, 361 (1989).
[2] E. Luijten and H. W. Blöte, Monte Carlo method for spin models with long-range interactions, Int. J. Mod. Phys. C **6**, 359

(1995).
[3] R. H. Swendsen and J.-S. Wang, Replica Monte Carlo Simulation of Spin-Glasses, Physical Review Letters **57**, 2607 (1986).
[4] E. Marinari and G. Parisi, Simulated Tempering: A New Monte Carlo Scheme, Europhysics Letters (EPL) **19**, 451 (1992).
[5] K. Hukushima and K. Nemoto, Exchange Monte Carlo Method and Application to Spin Glass Simulations, Journal of the Physical Society of Japan **65**, 1604 (1996).
[6] E. Granato, Zero-temperature transition and correlation-length exponent of the frustrated X Y model on a honeycomb lattice, Physical Review B **85**, 054508 (2012).
[7] J. M. Kosterlitz and D. J. Thouless, Ordering, metastability and phase transitions in two-dimensional systems, J. Phys. C: Solid State Phys. **6**, 1181 (1973).
[8] N. D. Mermin and H. Wagner, Absence of ferromagnetism or antiferromagnetism in one- or two-dimensional isotropic Heisenberg models, Phys. Rev. Lett. **17**, 1133 (1966).
[9] U. Schollwöck, T. Jolicœur, and T. Garel, Onset of incommensurability at the valence-bond-solid point in the $S$ =1 quantum spin chain, Phys. Rev. B **53**, 3304 (1996).
